# Supplementary material for: Chaotic dynamics of magnetic domain walls in nanowires
Source: arXiv:1604.04438 source file (2016-04-15)
Supplement: Supplementary file 1 [file Supplemental_Material.pdf]

# Chaotic dynamics of magnetic domain walls in nanowires – Supplemental Material

A. Pivano[1] and V.O. Dolocan[1, a)]

*Aix-Marseille Université, CNRS, IM2NP UMR7334, F-13397 Marseille Cedex 20, France*

[a)]Electronic mail: voicu.dolocan@im2np.fr

# I. DEPENDENCE OF CHAOTIC MOVEMENT ON THE MAGNETIC PARAMETERS

When the saturation magnetization $M_s$ is varied, the potential pinning energy changes as shown in Fig. S1(a) for a Py nanostrip with notches. The curvature and the potential barrier between the two wells vary. This changes the phase diagram of the DW motion, as shown in Fig. S2 for two values of $M_s$ larger and smaller than the usual Py value which is presented in the main text. The modification of the potential pinning energy, when the exchange constant A is varied, is shown in Fig. S1(b) for the same nanowire.

The potential pinning energy dependence on varying $M_s$ or A is shown in Fig. S1(c) and (d) for a Py nanostrip with two antinotches.

The phase diagram for a Ni nanostrip with notches is shown in Fig. S3 for a damping

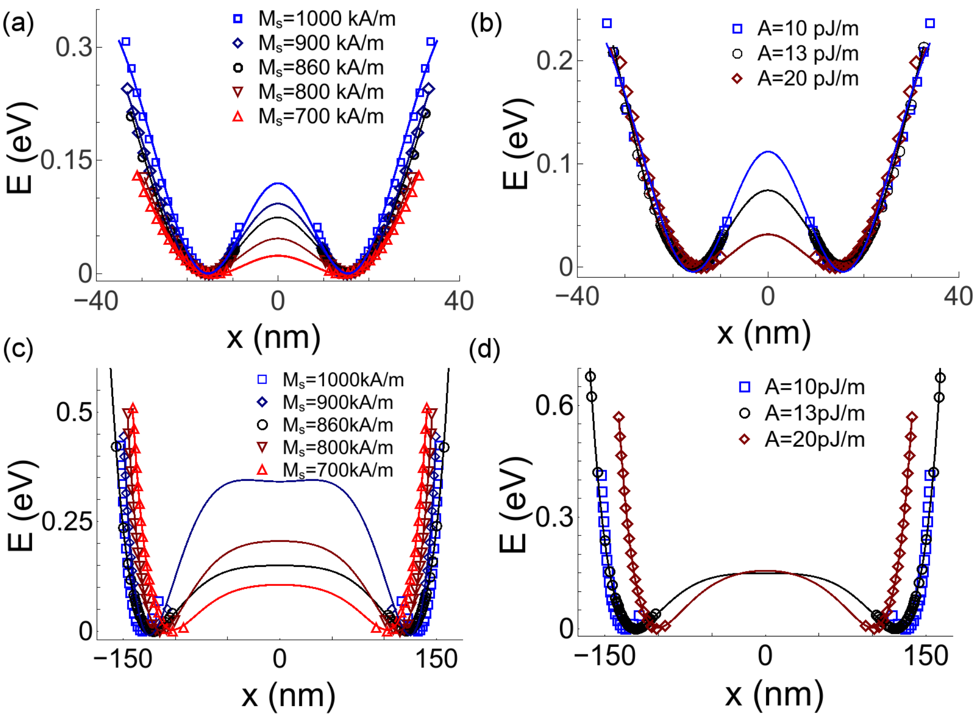


FIG. S1. (Color online) Variation of the potential pinning energy for a Py stripe with notches when the $M_s$ is varied (a) or the exchange constant A is varied (b). Variation of the potential pinning energy for a Py stripe with antinotches when the $M_s$ is varied (c) or the exchange constant A is varied (d). The lines are fits with same functions as used in the main text, but in some cases these functions don't work anymore (guide to the eyes).

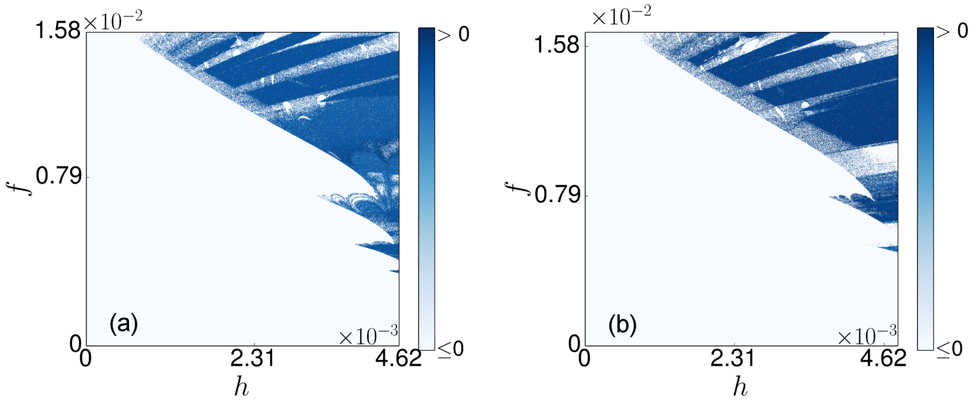


FIG. S2. (Color online) Normalized Lyapunov phase diagram for a DW at T=0K in a Py nanostrip with two double notches. Dark color represents chaotic motion. The parameters used are of Py with the exception of the saturation magnetization that was modified: (a) $M_s$ = 800kA/m and (b) $M_s$ = 900kA/m. The frequency $f$ is given in units of $\gamma_0 M_s$, which corresponds to an absolute scale of 0-2.79GHz for $M_s$ = 800kA/m and 0-3.14GHz for $M_s$ = 900kA/m. The amplitude of the applied field $h$ is given in units of $M_s$, that corresponds to 0-46.5Oe for $M_s$ = 800kA/m and to 0-52.3Oe for $M_s$ = 900kA/m. They are to be compared to the actual $M_s$ value (860kA/m) used in Fig.3(a) of the main text. Same field and frequency step were used in all diagrams, so the number of points in the above diagrams is not the same.

parameter $\alpha$=0.1 which is closer to the expected low temperature value than $\alpha$=0.02 which corresponds to the room temperature value.

## II. MICROMAGNETIC SIMULATIONS – VIDEOS

Four videos are presented with their names self-explanatory:

- two videos that present a periodic (period-3) and chaotic movement of DW in a Py nanowire with notches at 2.5GHz. The type of movement is shown in the bifurcation diagram of Fig.3(b) of the main text with the chaotic movement corresponding to the attractor shown in Fig.3(c).
- two videos that present chaotic movement in a nanowire with antinotches: one in a Py nanowire at 1GHz and 25Oe (see Fig.2(c) main text) and one in a Ni nanowire at 500MHz and 6Oe (see Fig.2(f) and (g) main text).

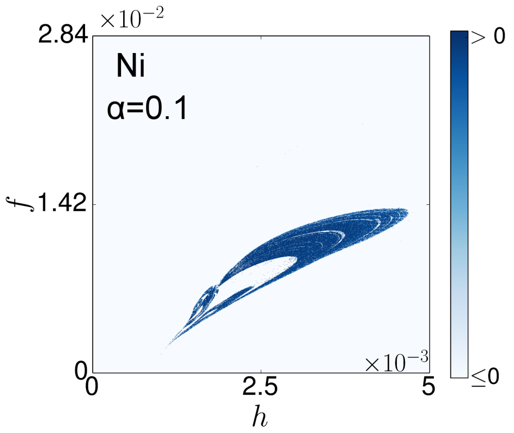


FIG. S3. (Color online) Normalized Lyapunov phase diagram for a DW at T=0K in a Ni nanostrip with two double notches. Dark color represents chaotic motion. The frequency $f$ is given in units of $\gamma_0 \mathrm{M}_s$, which corresponds to an absolute scale of 0-3GHz. The amplitude of the applied field $h$ is given in units of $\mathrm{M}_s$, that corresponds to 0-30Oe. The damping parameter $\alpha$ is 0.1. Fig.3(d) of the main text shows the same diagram for $\alpha = 0.02$.

All the videos are 20s long that corresponds to 40 periods of the applied magnetic field.
